# Supplementary material for: Representation Learning for Equivariant Inference with Guarantees
Source: arXiv:2505.19809 source file (2026-06-29)
Supplement: Supplementary file 1 [file checklist.tex]

\begin{enumerate}

    \item {\bf Claims}
        \item[] Question: Do the main claims made in the abstract and introduction accurately reflect the paper's contributions and scope?
        \item[] Answer: \answerYes{} % Replace by \answerYes{}, \answerNo{}, or \answerNA{}.
        \item[] Justification: Claims are new equivariant representation learning framework with theoretical guarantees and good performance in robotics applications. The method is presented in Section 4, the promised theoretical guarantees in Section 5, and the robotics applications in Section 6. % \justificationTODO{}
        \item[] Guidelines:
        \begin{itemize}
            \item The answer NA means that the abstract and introduction do not include the claims made in the paper.
            \item The abstract and/or introduction should clearly state the claims made, including the contributions made in the paper and important assumptions and limitations. A No or NA answer to this question will not be perceived well by the reviewers. 
            \item The claims made should match theoretical and experimental results, and reflect how much the results can be expected to generalize to other settings. 
            \item It is fine to include aspirational goals as motivation as long as it is clear that these goals are not attained by the paper. 
        \end{itemize}
    
    \item {\bf Limitations}
        \item[] Question: Does the paper discuss the limitations of the work performed by the authors?
        \item[] Answer: \answerYes{} % Replace by \answerYes{}, \answerNo{}, or \answerNA{}.
        \item[] Justification: We discuss in experiment section and conclusions that our method is data hungry and requires the finite symmetry group to be specified a priori.
        \item[] Guidelines:
        \begin{itemize}
            \item The answer NA means that the paper has no limitation while the answer No means that the paper has limitations, but those are not discussed in the paper. 
            \item The authors are encouraged to create a separate "Limitations" section in their paper.
            \item The paper should point out any strong assumptions and how robust the results are to violations of these assumptions (e.g., independence assumptions, noiseless settings, model well-specification, asymptotic approximations only holding locally). The authors should reflect on how these assumptions might be violated in practice and what the implications would be.
            \item The authors should reflect on the scope of the claims made, e.g., if the approach was only tested on a few datasets or with a few runs. In general, empirical results often depend on implicit assumptions, which should be articulated.
            \item The authors should reflect on the factors that influence the performance of the approach. For example, a facial recognition algorithm may perform poorly when image resolution is low or images are taken in low lighting. Or a speech-to-text system might not be used reliably to provide closed captions for online lectures because it fails to handle technical jargon.
            \item The authors should discuss the computational efficiency of the proposed algorithms and how they scale with dataset size.
            \item If applicable, the authors should discuss possible limitations of their approach to address problems of privacy and fairness.
            \item While the authors might fear that complete honesty about limitations might be used by reviewers as grounds for rejection, a worse outcome might be that reviewers discover limitations that aren't acknowledged in the paper. The authors should use their best judgment and recognize that individual actions in favor of transparency play an important role in developing norms that preserve the integrity of the community. Reviewers will be specifically instructed to not penalize honesty concerning limitations.
        \end{itemize}
    
    \item {\bf Theory assumptions and proofs}
        \item[] Question: For each theoretical result, does the paper provide the full set of assumptions and a complete (and correct) proof?
        \item[] Answer: \answerYes{} %\answerTODO{} % Replace by \answerYes{}, \answerNo{}, or \answerNA{}.
        \item[] Justification: We fully state assumptions and provide full proofs in the extensive appendices.% \justificationTODO{}
        \item[] Guidelines:
        \begin{itemize}
            \item The answer NA means that the paper does not include theoretical results. 
            \item All the theorems, formulas, and proofs in the paper should be numbered and cross-referenced.
            \item All assumptions should be clearly stated or referenced in the statement of any theorems.
            \item The proofs can either appear in the main paper or the supplemental material, but if they appear in the supplemental material, the authors are encouraged to provide a short proof sketch to provide intuition. 
            \item Inversely, any informal proof provided in the core of the paper should be complemented by formal proofs provided in appendix or supplemental material.
            \item Theorems and Lemmas that the proof relies upon should be properly referenced. 
        \end{itemize}
    
        \item {\bf Experimental result reproducibility}
        \item[] Question: Does the paper fully disclose all the information needed to reproduce the main experimental results of the paper to the extent that it affects the main claims and/or conclusions of the paper (regardless of whether the code and data are provided or not)?
        \item[] Answer: \answerYes{} % \answerTODO{} % Replace by \answerYes{}, \answerNo{}, or \answerNA{}.
        \item[] Justification: We will provide access to all the code and data used, along with clear explanations on how to reproduce the figures and tables in our paper. With extended details covered in appendix.% \justificationTODO{}
        \item[] Guidelines:
        \begin{itemize}
            \item The answer NA means that the paper does not include experiments.
            \item If the paper includes experiments, a No answer to this question will not be perceived well by the reviewers: Making the paper reproducible is important, regardless of whether the code and data are provided or not.
            \item If the contribution is a dataset and/or model, the authors should describe the steps taken to make their results reproducible or verifiable. 
            \item Depending on the contribution, reproducibility can be accomplished in various ways. For example, if the contribution is a novel architecture, describing the architecture fully might suffice, or if the contribution is a specific model and empirical evaluation, it may be necessary to either make it possible for others to replicate the model with the same dataset, or provide access to the model. In general. releasing code and data is often one good way to accomplish this, but reproducibility can also be provided via detailed instructions for how to replicate the results, access to a hosted model (e.g., in the case of a large language model), releasing of a model checkpoint, or other means that are appropriate to the research performed.
            \item While NeurIPS does not require releasing code, the conference does require all submissions to provide some reasonable avenue for reproducibility, which may depend on the nature of the contribution. For example
            \begin{enumerate}
                \item If the contribution is primarily a new algorithm, the paper should make it clear how to reproduce that algorithm.
                \item If the contribution is primarily a new model architecture, the paper should describe the architecture clearly and fully.
                \item If the contribution is a new model (e.g., a large language model), then there should either be a way to access this model for reproducing the results or a way to reproduce the model (e.g., with an open-source dataset or instructions for how to construct the dataset).
                \item We recognize that reproducibility may be tricky in some cases, in which case authors are welcome to describe the particular way they provide for reproducibility. In the case of closed-source models, it may be that access to the model is limited in some way (e.g., to registered users), but it should be possible for other researchers to have some path to reproducing or verifying the results.
            \end{enumerate}
        \end{itemize}
    
    
    \item {\bf Open access to data and code}
        \item[] Question: Does the paper provide open access to the data and code, with sufficient instructions to faithfully reproduce the main experimental results, as described in supplemental material?
        \item[] Answer: \answerYes{} % \answerTODO{} % Replace by \answerYes{}, \answerNo{}, or \answerNA{}.
        \item[] Justification: We will provide access to all code and data used for the paper. % \justificationTODO{}
        \item[] Guidelines:
        \begin{itemize}
            \item The answer NA means that paper does not include experiments requiring code.
            \item Please see the NeurIPS code and data submission guidelines (\url{https://nips.cc/public/guides/CodeSubmissionPolicy}) for more details.
            \item While we encourage the release of code and data, we understand that this might not be possible, so “No” is an acceptable answer. Papers cannot be rejected simply for not including code, unless this is central to the contribution (e.g., for a new open-source benchmark).
            \item The instructions should contain the exact command and environment needed to run to reproduce the results. See the NeurIPS code and data submission guidelines (\url{https://nips.cc/public/guides/CodeSubmissionPolicy}) for more details.
            \item The authors should provide instructions on data access and preparation, including how to access the raw data, preprocessed data, intermediate data, and generated data, etc.
            \item The authors should provide scripts to reproduce all experimental results for the new proposed method and baselines. If only a subset of experiments are reproducible, they should state which ones are omitted from the script and why.
            \item At submission time, to preserve anonymity, the authors should release anonymized versions (if applicable).
            \item Providing as much information as possible in supplemental material (appended to the paper) is recommended, but including URLs to data and code is permitted.
        \end{itemize}
    
    
    \item {\bf Experimental setting/details}
        \item[] Question: Does the paper specify all the training and test details (e.g., data splits, hyperparameters, how they were chosen, type of optimizer, etc.) necessary to understand the results?
        \item[] Answer: \answerYes{} % \answerTODO{} % Replace by \answerYes{}, \answerNo{}, or \answerNA{}.
        \item[] Justification: We provide experimental details in the corresponding appendix. % \justificationTODO{}
        \item[] Guidelines:
        \begin{itemize}
            \item The answer NA means that the paper does not include experiments.
            \item The experimental setting should be presented in the core of the paper to a level of detail that is necessary to appreciate the results and make sense of them.
            \item The full details can be provided either with the code, in appendix, or as supplemental material.
        \end{itemize}
    
    \item {\bf Experiment statistical significance}
        \item[] Question: Does the paper report error bars suitably and correctly defined or other appropriate information about the statistical significance of the experiments?
        \item[] Answer: \answerYes{} % \answerTODO{} % Replace by \answerYes{}, \answerNo{}, or \answerNA{}.
        \item[] Justification: We provided error bars. % \justificationTODO{}
        \item[] Guidelines:
        \begin{itemize}
            \item The answer NA means that the paper does not include experiments.
            \item The authors should answer "Yes" if the results are accompanied by error bars, confidence intervals, or statistical significance tests, at least for the experiments that support the main claims of the paper.
            \item The factors of variability that the error bars are capturing should be clearly stated (for example, train/test split, initialization, random drawing of some parameter, or overall run with given experimental conditions).
            \item The method for calculating the error bars should be explained (closed form formula, call to a library function, bootstrap, etc.)
            \item The assumptions made should be given (e.g., Normally distributed errors).
            \item It should be clear whether the error bar is the standard deviation or the standard error of the mean.
            \item It is OK to report 1-sigma error bars, but one should state it. The authors should preferably report a 2-sigma error bar than state that they have a 96\% CI, if the hypothesis of Normality of errors is not verified.
            \item For asymmetric distributions, the authors should be careful not to show in tables or figures symmetric error bars that would yield results that are out of range (e.g. negative error rates).
            \item If error bars are reported in tables or plots, The authors should explain in the text how they were calculated and reference the corresponding figures or tables in the text.
        \end{itemize}
    
    \item {\bf Experiments compute resources}
        \item[] Question: For each experiment, does the paper provide sufficient information on the computer resources (type of compute workers, memory, time of execution) needed to reproduce the experiments?
        \item[] Answer: \answerYes{} % Replace by \answerYes{}, \answerNo{}, or \answerNA{}.
        \item[] Justification: See experimental appendix.
        \item[] Guidelines:
        \begin{itemize}
            \item The answer NA means that the paper does not include experiments.
            \item The paper should indicate the type of compute workers CPU or GPU, internal cluster, or cloud provider, including relevant memory and storage.
            \item The paper should provide the amount of compute required for each of the individual experimental runs as well as estimate the total compute. 
            \item The paper should disclose whether the full research project required more compute than the experiments reported in the paper (e.g., preliminary or failed experiments that didn't make it into the paper). 
        \end{itemize}
        
    \item {\bf Code of ethics}
        \item[] Question: Does the research conducted in the paper conform, in every respect, with the NeurIPS Code of Ethics \url{https://neurips.cc/public/EthicsGuidelines}?
        \item[] Answer: \answerYes{} % Replace by \answerYes{}, \answerNo{}, or \answerNA{}.
        \item[] Justification: % \justificationTODO{}
        \item[] Guidelines:
        \begin{itemize}
            \item The answer NA means that the authors have not reviewed the NeurIPS Code of Ethics.
            \item If the authors answer No, they should explain the special circumstances that require a deviation from the Code of Ethics.
            \item The authors should make sure to preserve anonymity (e.g., if there is a special consideration due to laws or regulations in their jurisdiction).
        \end{itemize}
    
    
    \item {\bf Broader impacts}
        \item[] Question: Does the paper discuss both potential positive societal impacts and negative societal impacts of the work performed?
        \item[] Answer: \answerNA{} % Replace by \answerYes{}, \answerNo{}, or \answerNA{}.
        \item[] Justification: This paper mainly contributes theoretical/methodological results which have no direct societal impact. %\justificationTODO{}
        \item[] Guidelines:
        \begin{itemize}
            \item The answer NA means that there is no societal impact of the work performed.
            \item If the authors answer NA or No, they should explain why their work has no societal impact or why the paper does not address societal impact.
            \item Examples of negative societal impacts include potential malicious or unintended uses (e.g., disinformation, generating fake profiles, surveillance), fairness considerations (e.g., deployment of technologies that could make decisions that unfairly impact specific groups), privacy considerations, and security considerations.
            \item The conference expects that many papers will be foundational research and not tied to particular applications, let alone deployments. However, if there is a direct path to any negative applications, the authors should point it out. For example, it is legitimate to point out that an improvement in the quality of generative models could be used to generate deepfakes for disinformation. On the other hand, it is not needed to point out that a generic algorithm for optimizing neural networks could enable people to train models that generate Deepfakes faster.
            \item The authors should consider possible harms that could arise when the technology is being used as intended and functioning correctly, harms that could arise when the technology is being used as intended but gives incorrect results, and harms following from (intentional or unintentional) misuse of the technology.
            \item If there are negative societal impacts, the authors could also discuss possible mitigation strategies (e.g., gated release of models, providing defenses in addition to attacks, mechanisms for monitoring misuse, mechanisms to monitor how a system learns from feedback over time, improving the efficiency and accessibility of ML).
        \end{itemize}
        
    \item {\bf Safeguards}
        \item[] Question: Does the paper describe safeguards that have been put in place for responsible release of data or models that have a high risk for misuse (e.g., pretrained language models, image generators, or scraped datasets)?
        \item[] Answer: \answerNA{} % Replace by \answerYes{}, \answerNo{}, or \answerNA{}.
        \item[] Justification: See previous answer. % \justificationTODO{}
        \item[] Guidelines:
        \begin{itemize}
            \item The answer NA means that the paper poses no such risks.
            \item Released models that have a high risk for misuse or dual-use should be released with necessary safeguards to allow for controlled use of the model, for example by requiring that users adhere to usage guidelines or restrictions to access the model or implementing safety filters. 
            \item Datasets that have been scraped from the Internet could pose safety risks. The authors should describe how they avoided releasing unsafe images.
            \item We recognize that providing effective safeguards is challenging, and many papers do not require this, but we encourage authors to take this into account and make a best faith effort.
        \end{itemize}
    
    \item {\bf Licenses for existing assets}
        \item[] Question: Are the creators or original owners of assets (e.g., code, data, models), used in the paper, properly credited and are the license and terms of use explicitly mentioned and properly respected?
        \item[] Answer: \answerYes{} % Replace by \answerYes{}, \answerNo{}, or \answerNA{}.
        \item[] Justification: All data used comes from synthetic experiments or robotic simulations conducted by one of the authors of this paper, and open access datasets.% \justificationTODO{}
        \item[] Guidelines:
        \begin{itemize}
            \item The answer NA means that the paper does not use existing assets.
            \item The authors should cite the original paper that produced the code package or dataset.
            \item The authors should state which version of the asset is used and, if possible, include a URL.
            \item The name of the license (e.g., CC-BY 4.0) should be included for each asset.
            \item For scraped data from a particular source (e.g., website), the copyright and terms of service of that source should be provided.
            \item If assets are released, the license, copyright information, and terms of use in the package should be provided. For popular datasets, \url{paperswithcode.com/datasets} has curated licenses for some datasets. Their licensing guide can help determine the license of a dataset.
            \item For existing datasets that are re-packaged, both the original license and the license of the derived asset (if it has changed) should be provided.
            \item If this information is not available online, the authors are encouraged to reach out to the asset's creators.
        \end{itemize}
    
    \item {\bf New assets}
        \item[] Question: Are new assets introduced in the paper well documented and is the documentation provided alongside the assets?
        \item[] Answer: \answerNA{} % Replace by \answerYes{}, \answerNo{}, or \answerNA{}.
        \item[] Justification: %\justificationTODO{}
        \item[] Guidelines:
        \begin{itemize}
            \item The answer NA means that the paper does not release new assets.
            \item Researchers should communicate the details of the dataset/code/model as part of their submissions via structured templates. This includes details about training, license, limitations, etc. 
            \item The paper should discuss whether and how consent was obtained from people whose asset is used.
            \item At submission time, remember to anonymize your assets (if applicable). You can either create an anonymized URL or include an anonymized zip file.
        \end{itemize}
    
    \item {\bf Crowdsourcing and research with human subjects}
        \item[] Question: For crowdsourcing experiments and research with human subjects, does the paper include the full text of instructions given to participants and screenshots, if applicable, as well as details about compensation (if any)? 
        \item[] Answer: \answerNA{} % Replace by \answerYes{}, \answerNo{}, or \answerNA{}.
        \item[] Justification:
        \item[] Guidelines:
        \begin{itemize}
            \item The answer NA means that the paper does not involve crowdsourcing nor research with human subjects.
            \item Including this information in the supplemental material is fine, but if the main contribution of the paper involves human subjects, then as much detail as possible should be included in the main paper. 
            \item According to the NeurIPS Code of Ethics, workers involved in data collection, curation, or other labor should be paid at least the minimum wage in the country of the data collector. 
        \end{itemize}
    
    \item {\bf Institutional review board (IRB) approvals or equivalent for research with human subjects}
        \item[] Question: Does the paper describe potential risks incurred by study participants, whether such risks were disclosed to the subjects, and whether Institutional Review Board (IRB) approvals (or an equivalent approval/review based on the requirements of your country or institution) were obtained?
        \item[] Answer: \answerNA{}{} % Replace by \answerYes{}, \answerNo{}, or \answerNA{}.
        \item[] Justification: % \justificationTODO{}
        \item[] Guidelines:
        \begin{itemize}
            \item The answer NA means that the paper does not involve crowdsourcing nor research with human subjects.
            \item Depending on the country in which research is conducted, IRB approval (or equivalent) may be required for any human subjects research. If you obtained IRB approval, you should clearly state this in the paper. 
            \item We recognize that the procedures for this may vary significantly between institutions and locations, and we expect authors to adhere to the NeurIPS Code of Ethics and the guidelines for their institution. 
            \item For initial submissions, do not include any information that would break anonymity (if applicable), such as the institution conducting the review.
        \end{itemize}
    
    \item {\bf Declaration of LLM usage}
        \item[] Question: Does the paper describe the usage of LLMs if it is an important, original, or non-standard component of the core methods in this research? Note that if the LLM is used only for writing, editing, or formatting purposes and does not impact the core methodology, scientific rigorousness, or originality of the research, declaration is not required.
        %this research? 
        \item[] Answer: \answerNA{}{} % Replace by \answerYes{}, \answerNo{}, or \answerNA{}.
        \item[] Justification: We only used LLMs as a tool for improving the flow of the text. Nonetheless, we double checked and sign-off on all the text contained in the paper. % \justificationTODO{}
        \item[] Guidelines:
        \begin{itemize}
            \item The answer NA means that the core method development in this research does not involve LLMs as any important, original, or non-standard components.
            \item Please refer to our LLM policy (\url{https://neurips.cc/Conferences/2025/LLM}) for what should or should not be described.
        \end{itemize}
    
    \end{enumerate}
    
